# Supplementary material for: Fast-Response Variable Frequency DC-DC Converters Using Switching Cycle Event-Driven Digital Control
Source: arXiv:2209.05272 source file (2022-09-09)
Supplement: Supplementary file 1 [file 7_appendix.tex]

\begin{appendices}

\section{Large-Signal Stability of Current-Mode \\ DC-DC Converters} \label{appendix:cmc_modeling}
The large-signal modeling approach we will introduce applies to all types of current-mode dc-dc converters. In this section, we take the current-mode buck converter using constant on\nobreakdash-time and current-mode boost converter using constant off\nobreakdash-time as two typical examples. Only the analysis results are exhibited and the detailed proofs can be found in \cite{Avestruz2022}.

\subsection{Current-Mode Buck Converter Using Constant On-Time}
Consider a class $\Sigma$ buck converter defined in \cite{Cui2018a}, the off\nobreakdash-time at steady state is denoted by $T_{\text{off}}$.
The time varying off\nobreakdash-time is bounded from above by
\begin{align} \label{eqn:toff_bd_buck}
    T^{\text{min}}_{\text{off}} \le t_{\text{off}}[n] \le T^{\text{max}}_{\text{off}},
\end{align}
The large-signal stability can be described by the following three propositions proved by \cite{Avestruz2022}:
%We made two reasonable assumptions for power electronics to simplify the %derivation: 

\begin{figure}
    \centering
    \includegraphics[scale = 1]{Current_block_gain.png}
    \caption{$g(\hat{\alpha}.\hat{\beta})$ is the function of sector bounds $[\hat{\alpha}.\hat{\beta}]$.}
    \label{fig:Current_block_gain}
\end{figure}

\begin{proposition}
Given the class $\Sigma$ buck converter modeled in \cite{Cui2018a}, the $\mathcal{L}_2$ gain from the sampled output voltage sequence $\{\tilde{v}[n]\}$ to one-cycle-delayed inductor current sequence $\{\tilde{i}^{p}_v[n]\}$ is bounded from above by
\begin{align}\label{egn:gamma_vi_buck}
    \Gamma_{v \to i} \le \frac{T_s^{\text{ss}}}{L} g(\hat{\alpha}, \hat{\beta}),
\end{align}
where $g(\hat{\alpha}, \hat{\beta})$ follows Fig.\,\ref{fig:Current_block_gain}, $T_s^{\text{ss}}$ is the steady-state switching period, 
\begin{align}
    T_s^{\text{ss}} & \triangleq T_{\text{on}} +  T_{\text{off}}.
\end{align}
\end{proposition}

% \begin{align}
%     T_s^{\text{ss}} &\triangleq T_{\text{on}} +  T_{\text{off}}^{\text{ss}}.
% \end{align}

\begin{proposition}
Given the class $\Sigma$ buck converter using constant on-time modeled in \cite{Cui2018a}, the $\mathcal{L}_2$ gain from the one-cycle-delayed inductor current sequence $\{\tilde{i}^{p}_v[n]\}$ to sampled output voltage sequence $\{\tilde{v}[n]\}$ is bounded from above by
\begin{align}
    \Gamma_{i \to v} &  \le \frac{R}{\left( 1 + \frac{T_{\text{on}}}{2\tau_2}\right)} \frac{T_s^{\text{max}}}{T_s^{\text{min}}},
\end{align}
where $T_s^{\text{min}}$ and $T_s^{\text{max}}$ are the shortest switching period and longest switching period, respectively, and $\tau_2$ is the $L/R$ time constant,
\begin{align}
    T_s^{\text{max}} & \triangleq T_{\text{on}} +  T_{\text{off}}^{\text{max}}, \\
    T_s^{\text{min}} & \triangleq T_{\text{on}} +  T_{\text{off}}^{\text{min}},\\
    \tau_2 &\triangleq \frac{L}{R}.
\end{align}
\end{proposition}
\begin{proposition}
The current control loop of the class $\Sigma$ buck converter using constant on-time current-mode control is globally asymptotically stable if 
\begin{align}
    & g(\hat{\alpha}, \hat{\beta}) < \left(\tau_2 + \frac{T_{\text{on}}}{2}\right)\frac{T_s^{\text{min}}}{T_s^{\text{max}}} \frac{1}{T_s^{ss}}\:\: \text{and}\\
   & T_s^{\text{max}}\left( 1 + \frac{T_{\text{on}}}{2\tau_2}\right) < \tau_1,
\end{align}
where $g(\hat{\alpha}, \hat{\beta})$ follows Fig.\,\ref{fig:Current_block_gain}, $T_s^{\text{min}}$ and $T_s^{\text{max}}$ are the shortest switching period and longest switching period, respectively,
$\tau_1$ is the $RC$ time constant, and $\tau_2$ is the $L/R$ time constant,
\begin{align}
    T_s^{\text{max}} & \triangleq T_{\text{on}} +  T_{\text{off}}^{\text{max}}, \\
    T_s^{\text{min}} & \triangleq T_{\text{on}} +  T_{\text{off}}^{\text{min}},\\
    \tau_1 &\triangleq RC, \\
    \tau_2 &\triangleq \frac{L}{R}.
\end{align}
\end{proposition}

\subsection{Current-Mode Boost Converter Using Constant Off-Time}
Consider a class $\Sigma$ boost converter using constant off-time defined in \cite{Cui2018a}, the on-time in steady state is denoted by $T_{\text{off}}$.
The time-varying on-time is bounded from above by
\begin{align} \label{eqn:toff_bd_boost}
    T^{\text{min}}_{\text{on}} \le t_{\text{on}}[n] \le T^{\text{max}}_{\text{on}}.
\end{align}
The large-signal stability can be described by the following three propositions proved by \cite{Avestruz2022}:
\begin{proposition}
Given the class $\Sigma$ boost converter using constant off-time control, the $\mathcal{L}_2$ gain from the sampled output voltage sequence $\{\tilde{v}[n]\}$ to one-cycle-delayed inductor current sequence $\{\tilde{i}^{p}_p[n]\}$ is bounded from above by
\begin{align}\label{egn:gamma_vi_boost}
    \Gamma_{v \to i} \le \frac{T_{\text{off}}}{L} g(\hat{\alpha}, \hat{\beta}),
\end{align}
where $g(\hat{\alpha}, \hat{\beta})$ follows Fig.\,\ref{fig:Current_block_gain}, $T_s^{\text{ss}}$ is the steady-state switching period, 
\begin{align}
    T_s^{\text{ss}} & \triangleq T_{\text{on}} +  T_{\text{off}}.
\end{align}
\end{proposition}

\begin{proposition}
Given the class $\Sigma$ boost converter using constant off-time control, the $\mathcal{L}_2$ gain from the one-cycle-delayed inductor current sequence $\{\tilde{i}^{p}_p[n]\}$ to sampled output voltage sequence $\{\tilde{v}[n]\}$ is bounded from above by the following:

\vspace{+8pt}
\noindent (i) if $\left((1-\lambda ) T_{\text{off}} + \frac{V_{\text{out}}L}{V_{\text{in}}R} \right)\left( 1-\frac{T_s^{\text{ss}}}{RC} -\frac{T_{s}^{\text{max}}}{RC}-\frac{ T^2_{\text{off}}}{2LC}\right) + \left( \lambda T_{\text{off}} - \frac{V_{\text{out}}L}{V_{\text{in}}R} \right) \ge 0 $\:\:and
\begin{align} \label{eqn:ivgain_case1_cotcm}
    \Gamma_{i \to v} &  \le \frac{R}{\left( \frac{T_s^{\text{ss}} + T_s^{\text{min}}}{T_{\text{off}}} + \frac{T_{\text{off}}}{2\tau_2}\right)},
\end{align}

\noindent or (ii) if $\left((1-\lambda ) T_{\text{off}} + \frac{V_{\text{out}}L}{V_{\text{in}}R} \right)\left( 1-\frac{T_s^{\text{ss}}}{RC} -\frac{T_{s}^{\text{max}}}{RC}-\frac{ T^2_{\text{off}}}{2LC}\right) + \left( \lambda T_{\text{off}} - \frac{V_{\text{out}}L}{V_{\text{in}}R} \right) < 0 $\:\:and
\begin{align} \label{eqn:ivgain_case2_cotcm}
    \Gamma_{i \to v} &  \le \frac{2\tau_2\left( T_s^{\text{max}} +  T_s^{\text{ss}}\right) + T_{\text{off}}^2}{2\tau_2\left( T_s^{\text{min}} +  T_s^{\text{ss}}\right) + T_{\text{off}}^2} \frac{2\tau_2\frac{V_{\text{out}}}{V_{\text{in}}}+(1-2\lambda)T_{\text{off}}}{2\tau_1-T_s^{\text{ss}}-T_s^{\text{max}}-\frac{T_{\text{off}}^2}{2\tau_2}} R,
\end{align}
where $T_s^{\text{min}}$ and $T_s^{\text{max}}$ are the shortest switching period and longest switching period, respectively, $\tau_1$ is the $RC$ time constant, and $\tau_2$ is the $L/R$ time constant,
\begin{align}
    T_s^{\text{max}} & \triangleq T_{\text{off}} +  T_{\text{on}}^{\text{max}}, \\
    T_s^{\text{min}} & \triangleq T_{\text{off}} +  T_{\text{on}}^{\text{min}}, \\
    \tau_1 &\triangleq RC, \\
    \tau_2 &\triangleq \frac{L}{R}.
\end{align}
\end{proposition}

\begin{proposition}\label{theore: boost_offtime_stability_cotcmboost}
The current control loop of the class $\Sigma$ boost converter using constant off-time control is globally asymptotically stable

\vspace{+8pt}
\noindent (i) if $\left((1-\lambda ) T_{\text{off}} + \frac{V_{\text{out}}L}{V_{\text{in}}R} \right)\left( 1-\frac{T_s^{\text{ss}}}{RC} -\frac{T_{s}^{\text{max}}}{RC}-\frac{ T^2_{\text{off}}}{2LC}\right) + \left( \lambda T_{\text{off}} - \frac{V_{\text{out}}L}{V_{\text{in}}R} \right) \ge 0 $\:\:and
\begin{align}
    g(\hat{\alpha}, \hat{\beta}) &  \le 
    \frac{1}{2} + \tau_2
   \left(\frac{T_s^{\text{ss}}+T_s^{\text{min}}}{T_s^{\text{ss}}T_{\text{off}}} \right);
\end{align}

\noindent or (ii) if $\left((1-\lambda ) T_{\text{off}} + \frac{V_{\text{out}}L}{V_{\text{in}}R} \right)\left( 1-\frac{T_s^{\text{ss}}}{RC} -\frac{T_{s}^{\text{max}}}{RC}-\frac{ T^2_{\text{off}}}{2LC}\right) + \left( \lambda T_{\text{off}} - \frac{V_{\text{out}}L}{V_{\text{in}}R} \right) < 0 $\:\:and
\begin{align}
    &g(\hat{\alpha}, \hat{\beta}) \le\\\nonumber
    &\frac{2\tau_2\left( T_s^{\text{min}} +  T_s^{\text{ss}}\right) + T_{\text{off}}^2}{2\tau_2\left( T_s^{\text{max}} +  T_s^{\text{ss}}\right) + T_{\text{off}}^2} \frac{2\tau_1-T_s^{\text{ss}}-T_s^{\text{max}}-\frac{T_{\text{off}}^2}{2\tau_2}}{2\frac{V_{\text{out}}}{V_{\text{in}}}+(1-2\lambda)\frac{T_{\text{off}}}{\tau_2}}T_{\text{off}};
\end{align}
where $g(\hat{\alpha}, \hat{\beta})$ follows Fig.\,\ref{fig:Current_block_gain}, $T_s^{\text{min}}$ and $T_s^{\text{max}}$ are the shortest switching period and longest switching period, respectively, $\tau_1$ is the $RC$ time constant, and $\tau_2$ is the $L/R$ time constant,
\begin{align}
    T_s^{\text{max}} & \triangleq T_{\text{on}} +  T_{\text{off}}^{\text{max}}, \\
    T_s^{\text{min}} & \triangleq T_{\text{on}} +  T_{\text{off}}^{\text{min}},\\
    \tau_1 &\triangleq RC, \\
    \tau_2 &\triangleq \frac{L}{R}.
\end{align}
\end{proposition}

\section{Design Equations for Three Other Typical Current-Mode Converters} \label{ref:sec_design_eqn}
We directly use the settling $N_w$ as the metric for settling cycles,
\begin{align} \label{eqn:settlecycle_repeat}
    N_w \triangleq \text{max} \bigg\{\bigg|\frac{4}{\text{ln}(|a_{\text{min}}|)}\bigg|,\bigg|\frac{4}{\text{ln}(|a_{\text{max}}|)}\bigg|\bigg\}.
\end{align}
The worst-case overshoot $O_w$ follows
\begin{align} \label{eqn:os1p1z_repeat}
    O_w \triangleq \text{max}\bigg\{\frac{b-a_{\text{min}}}{1-b}\,,\,0\bigg\}.
\end{align}
The design equations of the constant on-time current-mode converter, constant off-time current-mode converter, fixed-frequency peak current-mode converter and fixed-frequency valley current-mode converter are illustrated in Tables\,\ref{table:cont_off_cm_theory},
\ref{table:cofft_on_cm_theory}, 
\ref{table:ff_peak_cm_theory}, and \ref{table:ff_valley_cm_theory}.
\begin{table*}[tb]
    \caption{Design Theory and Equations for Constant Off-Time Current-Mode Converters}
    \label{table:cont_off_cm_theory}
    \centering
    \begin{tabular}
    {|m{2.4in}|m{1.025in}|m{1.025in}|m{0.55in}|}
    %{|c|c|c|c||c|}
      %\toprule
        \hline
        \textbf{Stability Criteria} & $\mathbf{a_{\text{min}}}$ & $\mathbf{a_{\text{max}}}$ & \textbf{b} \\
        \hline
        \vspace{3pt}
        $\Lambda_{ub} \le \frac{m_1}{2}$
        \vspace{2pt}
        & $1 - \frac{m_1}{(m_1 - \Lambda_{ub})}$
        \vspace{2pt}
        & $1 - \frac{m_1}{(m_1 + \Lambda_{ub})}$
        \vspace{2pt}
        & 0 \\
        %\midrule
        %  \hline
        % \textbf{Slope \newline Compensation}
        % & $\Lambda_{ub} \le \frac{m_1}{2} + m_s $
        % & $\frac{m_s-\Lambda_{ub}}{(m_1 + m_s - \Lambda_{ub})}$
        % & $\frac{m_s+\Lambda_{ub}}{(m_1 + m_s + \Lambda_{ub})}$
        % & 0 \\
        %\midrule
        \hline
    \end{tabular}
\end{table*}

\begin{table*}[tb]
    \caption{Design Theory and Equations for the Constant On-Time Current-Mode Converters}
    \label{table:cofft_on_cm_theory}
    \centering
    \begin{tabular}
    {|m{2.4in}|m{1.025in}|m{1.025in}|m{0.55in}|}
    %{|c|c|c|c||c|}
      %\toprule
        \hline
        \textbf{Stability Criteria}& $\mathbf{a_{\text{min}}}$ & $\mathbf{a_{\text{max}}}$ & \textbf{b} \\
        %\midrule
        \hline
        \vspace{3pt}
        $\Lambda_{ub} \le \frac{m_2}{2}$
         \vspace{2pt}
        & $1 - \frac{m_2}{(m_2 - \Lambda_{ub})}$
         \vspace{2pt}
        & $1 - \frac{m_2}{(m_2 + \Lambda_{ub})}$
         \vspace{2pt}
        & 0 \\
        %\midrule
        %  \hline
        % \textbf{Slope \newline Compensation}
        % & $\Lambda_{ub} \le \frac{m_2}{2} + m_s $
        % & $\frac{m_s-\Lambda_{ub}}{(m_2 + m_s - \Lambda_{ub})}$
        % & $\frac{m_s+\Lambda_{ub}}{(m_2 + m_s + \Lambda_{ub})}$
        % & 0 \\
        %\midrule
         \hline
    \end{tabular}
\end{table*}

\begin{table*}[tb]
    \caption{Design Theory and Equations for the Fixed-Frequency Peak Current-Mode Converters}
    \label{table:ff_peak_cm_theory}
    \centering
    \begin{tabular}
    {|m{2.4in}|m{1.025in}|m{1.025in}|m{0.55in}|}
    %{|c|c|c|c||c|}
      %\toprule
        \hline
        \textbf{Stability Criteria}& $\mathbf{a_{\text{min}}}$ & $\mathbf{a_{\text{max}}}$ & \textbf{b} \\
        %\midrule
        \hline
        \vspace{3pt}
        $\Lambda_{ub} \le \frac{m_1 - m_2}{2}$ 
        \vspace{2pt}
        & $\frac{-\Lambda_{ub}-m_2}{(m_1 - \Lambda_{ub})}$
        \vspace{2pt}
        & $\frac{\Lambda_{ub} - m_2}{(m_1 + \Lambda_{ub})}$
        \vspace{2pt}
        & $-\frac{m_2}{m_1}$
        \vspace{2pt} \\
        %\midrule
        %  \hline
        % \textbf{Slope \newline Compensation}
        % & $\Lambda_{ub} \le \frac{m_1-m_2}{2} + m_s $
        % & $\frac{m_s-\Lambda_{ub}-m_2}{(m_1 + m_s - \Lambda_{ub})}$
        % & $\frac{m_s+\Lambda_{ub}-m_2}{(m_1 + m_s + \Lambda_{ub})}$
        % &  $-\frac{m_2}{m_1}$\\
        %\midrule
         \hline
    \end{tabular}
\end{table*}

\begin{table*}[tb]
    \caption{Design Theory and Equations for the Fixed-Frequency Valley Current-Mode Converters}
    \label{table:ff_valley_cm_theory}
    \centering
    \begin{tabular}
    {|m{2.4in}|m{1.025in}|m{1.025in}|m{0.55in}|}
    %{|c|c|c|c||c|}
      %\toprule
        \hline
        \textbf{Stability Criteria}& $\mathbf{a_{\text{min}}}$ & $\mathbf{a_{\text{max}}}$ & \textbf{b} \\
        %\midrule
        \hline
        \vspace{3pt}
        $\Lambda_{ub} \le \frac{m_2 - m_1}{2}$ 
        \vspace{2pt}
        & $\frac{-\Lambda_{ub}-m_1}{(m_2 - \Lambda_{ub})}$
        \vspace{2pt}
        & $\frac{\Lambda_{ub} - m_1}{(m_2 + \Lambda_{ub})}$
        \vspace{2pt}
        & $-\frac{m_1}{m_2}$ 
        \vspace{2pt}
        \\
        %\midrule
        %  \hline
        % \textbf{Slope \newline Compensation}
        % & $\Lambda_{ub} \le \frac{m_2-m_1}{2} + m_s $
        % & $\frac{m_s-\Lambda_{ub}-m_1}{(m_2 + m_s - \Lambda_{ub})}$
        % & $\frac{m_s+\Lambda_{ub}-m_1}{(m_2 + m_s + \Lambda_{ub})}$
        % &  $-\frac{m_1}{m_2}$\\
        %\midrule
         \hline
    \end{tabular}
\end{table*}

\section{Sector Boundedness of Static Mapping $\mathcal{T}$} \label{ref:sec_boun_Tmap}
\begin{proof}
We denote the bandwidth limit of interference $w(t)$ by $f_{ub}$ and amplitude limit of the interference by $A_{ub}$.
From Bernstein's inequality \cite{Lapidoth2009},
\begin{align}
    \Bigg | \frac{\text{d}\,w(t)}{\text{d}\,t} \Bigg |\le 4\pi f_{ub} A_{ub} \triangleq \Lambda_{ub}, \: \forall t \in \mathbb{R}.
\end{align}
We linearly transform the static mapping $\mathcal{T}$ to the origin, which results in $\tilde{\mathcal{T}}$
%  \begin{align}
%         \mathcal{T}:i_c & \rightarrow i_p  \label{eqn:defT_1},\\
%         \tilde{\mathcal{T}}: \tilde{i}_c & \rightarrow \tilde{i}_p \label{eqn:deftildeT_1},\\
%         \mathcal{T}(\tilde{i}_c) & = I_p + \tilde{\mathcal{T}}(i_c - Ic) \label{eqn:TtildeT_1},\\
%         \tilde{\mathcal{T}}(0) & = 0. \label{eqn:proptildeT_1}
% \end{align}
\begin{align}
    i_c  = I_c & + \tilde{i}_c,   \\
    i_p  = I_p & + \tilde{i}_p,   \\
    \mathcal{T}:i_c & \rightarrow i_p  \label{eqn:defT_2},\\
    \tilde{\mathcal{T}}: \tilde{i}_c & \rightarrow \tilde{i}_p \label{eqn:deftildeT_2}.
\end{align}
The relationship between $\tilde{\mathcal{T}}$ and $\psi$ follows
\begin{align}
        \frac{\text{d}\,(\tilde{\mathcal{T}}^{-1})}{\text{d}\,x}  & = 1 + G_0\psi^{'} \label{eqn:devTinvx_1},\:
        \text{where}\; \psi^{'} = \frac{\text{d}\,\psi(x)}{\text{d}\,x},\\
       \frac{\text{d}\,\tilde{\mathcal{T}}}{\text{d}\,x} & = \frac{1}{1 + G_0\psi^{'}}\label{eqn:devTx_1},
\end{align}
\begin{align}
         \psi^{'} & = \frac{1}{G_0} \left( \frac{1}{\frac{\text{d}\,\tilde{\mathcal{T}}}{\text{d}\,x}} - 1  \right) = \frac{1}{G_0} \left( \frac{1}{\frac{\text{d}\,\mathcal{T}}{\text{d}\,x}} - 1  \right) \label{eqn:devpsi_1}.
\end{align}
The relationship between $\psi(t)$ and $w(t)$ follows
\begin{align}
     \psi(t) & = w(t+T_{\text{on}}) - w(T_{\text{on}}) \label{eqn:psit_wt_1},\\
     \frac{\text{d}\,\psi(t)}{\text{d}\,t} & = \frac{\text{d}\,w(t)}{\text{d}\,t}, \\
     -\Lambda_{ub} \le  & \frac{\text{d}\,w(t)}{\text{d}\,t} \le  \Lambda_{ub} \label{eqn:dpsit_dwt_1}.
\end{align}
From (\ref{eqn:dpsit_dwt_1}) and (\ref{eqn:devTx_1})
\begin{align}
         \frac{1}{1 + \Lambda_{ub} G_0} \le \frac{\text{d}\,\tilde{\mathcal{T}}}{\text{d}\,x} \le \frac{1}{1 - \Lambda_{ub} G_0}   \label{eqn:devTx_1_1},
\end{align}
\begin{align}
     \tilde{\mathcal{T}}(x) = \tilde{\mathcal{T}}(x) -  \tilde{\mathcal{T}}(0) = \int_0^{x} \frac{\text{d} \tilde{\mathcal{T}}}{\text{d} x}\,\text{d} x. \label{eqn:boundTtilde}
\end{align}
Therefore, we have proven $\tilde{\mathcal{T}}$ is sector-bounded
\begin{align}
    \frac{x}{1 + \Lambda_{ub} G_0} \le \tilde{\mathcal{T}}(x) \le \frac{x}{1 - \Lambda_{ub} G_0}.
\end{align}
We have proven $\mathcal{T}$ is $\alpha$ sector-bounded with
\begin{align}
    \alpha &= I_p, \\
    K_{lb} &= \frac{1}{1 + \Lambda_{ub} G_0}, \quad 
    K_{ub} = \frac{1}{1 - \Lambda_{ub} G_0}.
\end{align}
\end{proof}

\section{Proof of Theorem \ref{th:equexcond}}  \label{proof:equexcond}
\begin{proof}
%To prove 
% \begin{enumerate}
% \item One if the measured inductor current waveform $m_{1}t+w(t)$ is strictly monotonic then $\mathcal{T}$ is onto function.
% \item Two if $\mathcal{T}$ is onto function then measured inductor current waveform $m_{1}t+w(t)$ is strictly monotonic.
% \end{enumerate}
If first-event-triggering with latching is used, $\mathcal{T}$ is a monotonically increasing mapping. Therefore, the proposition that $\mathcal{T}$ is continuous is equivalent to the proposition that $\mathcal{T}$ is onto. We first prove that if the current sensor output \mbox{$m_{1}t+w(t)$} is strictly monotonic, $\mathcal{T}$ is an onto mapping. We next prove that if $\mathcal{T}$ is an onto mapping, the current sensor output $m_{1}t+w(t)$ is strictly monotonic. The contradiction method is used in the proof.

1. The current sensor output $m_{1}t+w(t)$ is strictly \\
monotonic $\Longrightarrow$ $\mathcal{T}$ is an onto function.\\
Given any $I_p$, there uniquely exists an on-time $t_{\text{on}}$ which satisfies
\begin{align}
  I_{p}= I_{v} + m_{1}t_{\text{on}}.
\end{align}
% that is for $I_{p} \in R $, $ \exists $ $ $ $t_{\text{on}} \in T $  such that function G exists
% \begin{equation}
% \begin{aligned}
% G : I_P \rightarrow T\\ 
% G(I_{p}) = t_{\text{on}}
% \end{aligned}
% \end{equation}\\ 
Because the measured inductor current waveform $m_{1}t+w(t)$ is strictly monotonic, given any $t_{\text{on}}$, there uniquely exists a current command $I_c$ which achieves \,$t_{\text{on}}$ by following the first-event-triggering with latching mechanism
\begin{align}
I_c = I_v+m_{1}t_{\text{on}}+w(t_{\text{on}}),
\end{align}
where $I_{v}$ is the valley current. To consolidate, given any $I_p$, there uniquely exists a $t_{\text{on}}$ and given any $t_{\text{on}}$, there uniquely exists an $I_c$.
Therefore, we have proven that $\mathcal{T}$ is an onto function.

2. $\mathcal{T}$ is an onto function $\Longrightarrow$  the measured inductor current waveform $ m_{1}t+w(t)$ is strictly monotonic.\\
We prove it by contradiction. We assume that $m_{1}t+w(t)$ is not strictly monotonic, hence there exist $t_{\text{on1}}$ and $t_{\text{on2}}$ such that
\begin{equation}
\begin{aligned}
t_{\text{on2}} >  t_{\text{on1}} \Longrightarrow m_{1}t_{\text{on2}}+w(t_{\text{on2}}) \leq m_{1}t_{\text{on1}}+w(t_{\text{on1}}).
\end{aligned}
\end{equation}
The corresponding $I_{p1}$ of $t_{\text{on1}}$ and $I_{p2}$ of $t_{\text{on2}}$ are 
\begin{equation}
\begin{aligned}
I_{p1}= I_{v} + m_{1}t_{\text{on1}}, \quad  \quad I_{p2}= I_{v} + m_{1}t_{\text{on2}}. 
\end{aligned}
\end{equation}
% given $\mathcal{T}$ : $\mathbb{R}^n$ $\rightarrow$ $\mathbb{R}^n$ is mapping from the inductor current command $I_c$ to the actual inductor current $I_p$ in the steady state.\\
Because $\mathcal{T}$ is an onto function,
% for all $I_p \in \mathbb{R}^n $, there exists $I_c$ $\in$ $\mathbb{R}^n$ such that 
% \begin{equation}
% \begin{aligned}
% \mathcal{T}(I_c) = I_p.
% \end{aligned}
% \end{equation}
there exist $ I_{c1},I_{c2}$ such that
\begin{align}
    \mathcal{T}(I_{c1})= I_{p1}, \quad \quad
    \mathcal{T}(I_{c2})= I_{p2}.
\end{align}
From the definition of $I_{c1}$ and $I_{c2}$,
\begin{align}
    I_{c1} &= I_{v} + m_{1}t_{\text{on1}}+w(t_{\text{on1}}), \nonumber \\
    I_{c2} &= I_{v} + m_{1}t_{\text{on2}}+w(t_{\text{on2}}) \label{eqn:icexp}, 
\end{align}
where $I_{v}$ is the valley current. \\
Because of the first-event-trigger with latching mechanism, for $I_{c2} > I_{c1}$, we have  $t_{\text{on2}} > t_{\text{on1}}$. From (\ref{eqn:icexp}), we obtained
\begin{equation}
\begin{aligned}
 m_{1}t_{\text{on2}}+w(t_{\text{on2}}) > m_{1}t_{\text{on1}}+w(t_{\text{on1}}), \\
\end{aligned}
\end{equation}
% i.e for 
% \begin{equation}
% \begin{aligned}
% t_{on2} > t_{on1} \Longrightarrow m_{1}t_{on2}+f(t_{on2}) > m_{1}t_{on1}+f(t_{on1})
% \end{aligned}
% \end{equation}
which contradicts the assumption that $m_{1}t_{\text{on1}}+w(t_{\text{on1}})$ is not strictly monotonic. Hence we have proven that if $\mathcal{T}$ is an onto function, the measured inductor current waveform $m_{1}t+w(t)$ is strictly monotonic.
\end{proof}

\end{appendices}
